# Supplementary material for: Identification of stormwater control strategies and their associated uncertainties using Bayesian Optimization
Source: arXiv:2305.18630 source file (2023-05-29)
Supplement: Supplementary file 1 [file supplimentary.tex]

\documentclass[../bayesnew.tex]{subfiles}

\begin{document}
\section{Supplementary Information}

\subsection{Generalizability: Scenario Epsilon}

%Performance of the controller 
\end{document}
